# Supplementary material for: Efficient LLM Serving on Hybrid Real-time and Best-effort Requests
Source: arXiv:2504.09590 source file (2025-04-13)
Supplement: Supplementary file 1 [file old_Appendix.tex]

\clearpage
\section{Comparison on Hybrid Workloads}
\label{app:compare}
\begin{figure*}[!t]
    \centering
     \begin{subfigure}[b]{0.49\linewidth}
     \centering
     \includegraphics[width=\linewidth]{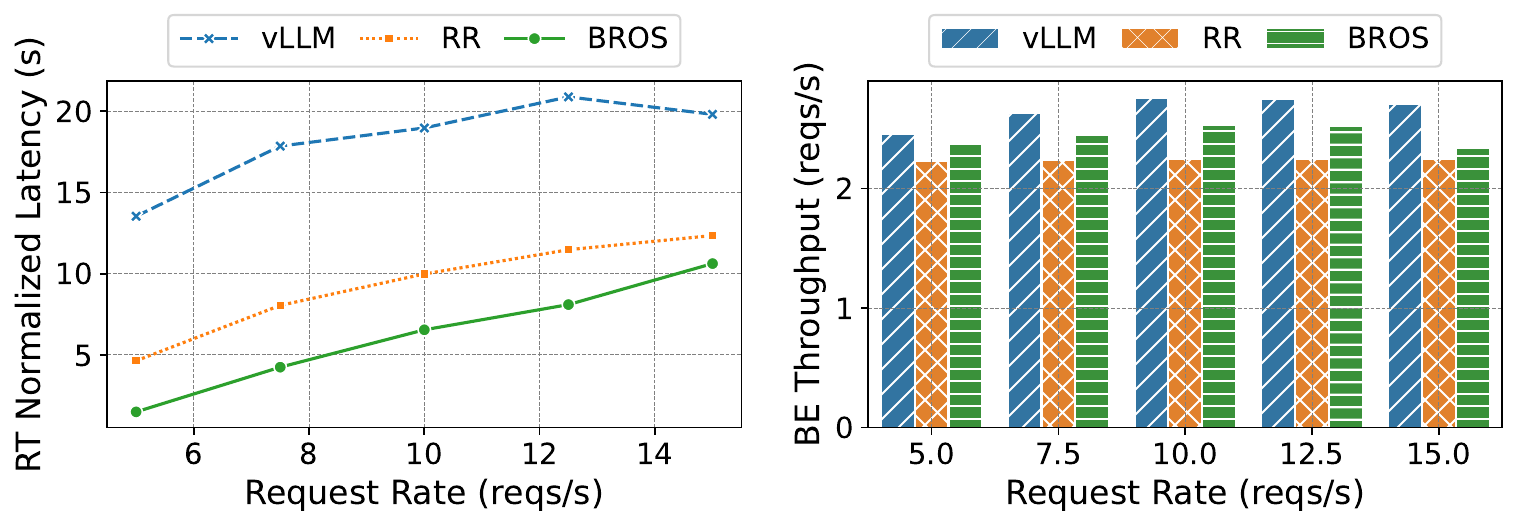}
     \caption{OPT-13B, 2GPUs, SharedGPT.}
     \label{fig:opt-13b-sharedgpt_latency_thp}
    \end{subfigure}
     \hfill
     \begin{subfigure}[b]{0.49\linewidth}
         \centering
         \includegraphics[width=\linewidth]{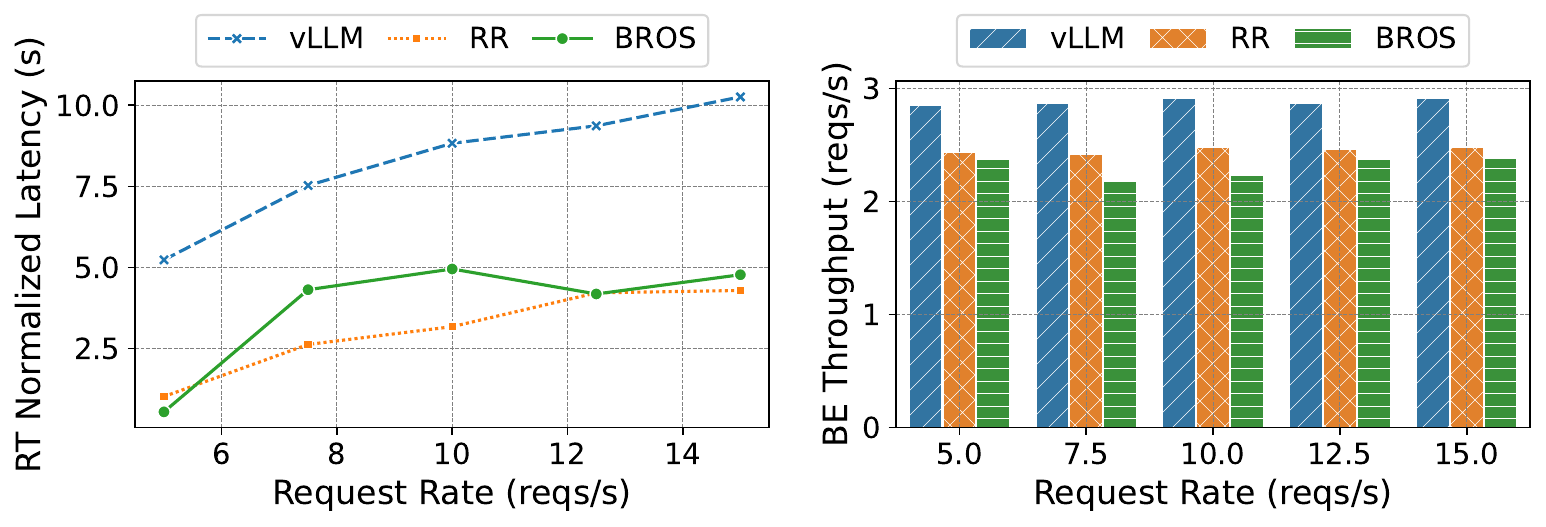}
         \caption{OPT-13B, 2GPUs, LMSYS-CHAT-1M.}
         \label{fig:opt-13b-lmsys-chat-1m_latency_thp}
     \end{subfigure}
      \hfill
     \begin{subfigure}[b]{0.49\linewidth}
         \centering
         \includegraphics[width=\linewidth]{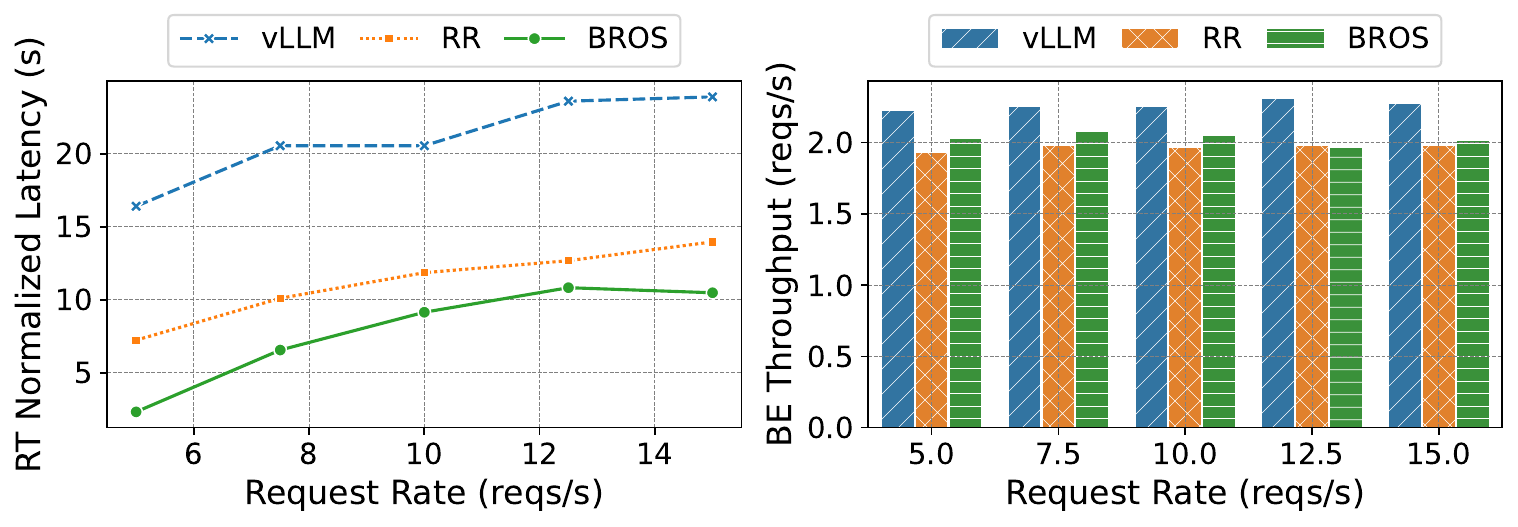}
         \caption{OPT-30B, 4GPUs, SharedGPT.}
         \label{fig:opt-30b-sharedgpt_latency_thp}
     \end{subfigure}
     \hfill
     \begin{subfigure}[b]{0.49\linewidth}
         \centering
         \includegraphics[width=\linewidth]{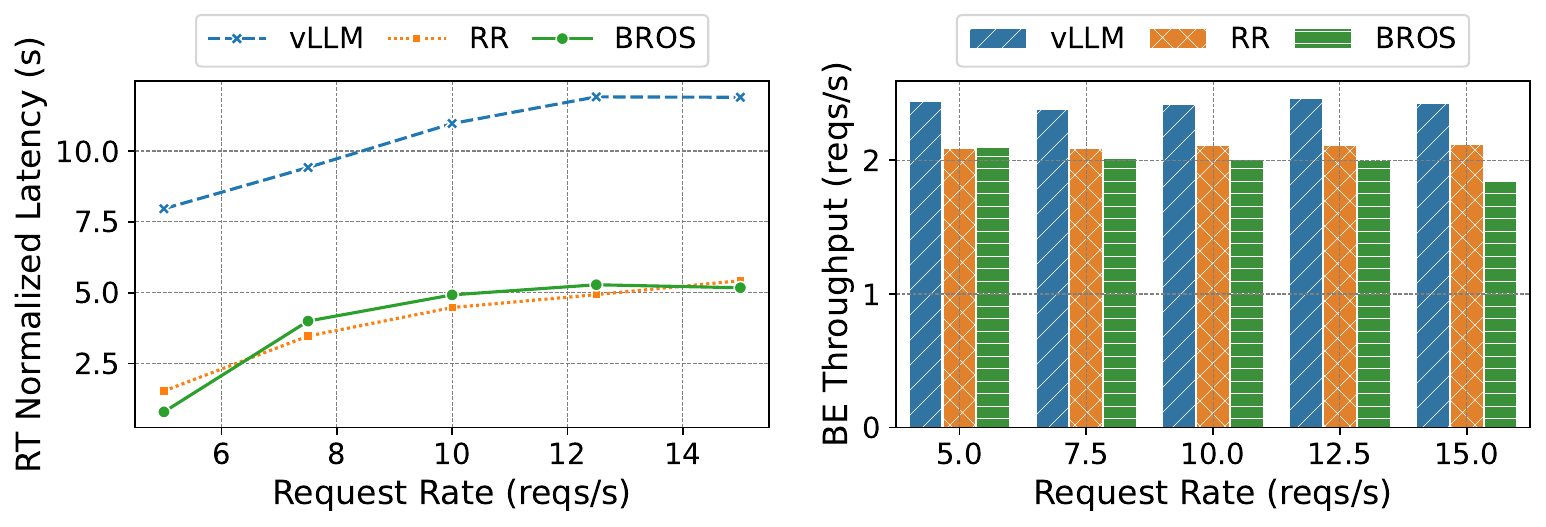}
         \caption{OPT-30B, 4GPUs, LMSYS-CHAT-1M.}
         \label{fig:opt-30b-lmsys-chat-1m_latency_thp}
     \end{subfigure}
     \hfill
     \begin{subfigure}[b]{0.49\linewidth}
         \centering
         \includegraphics[width=\linewidth]{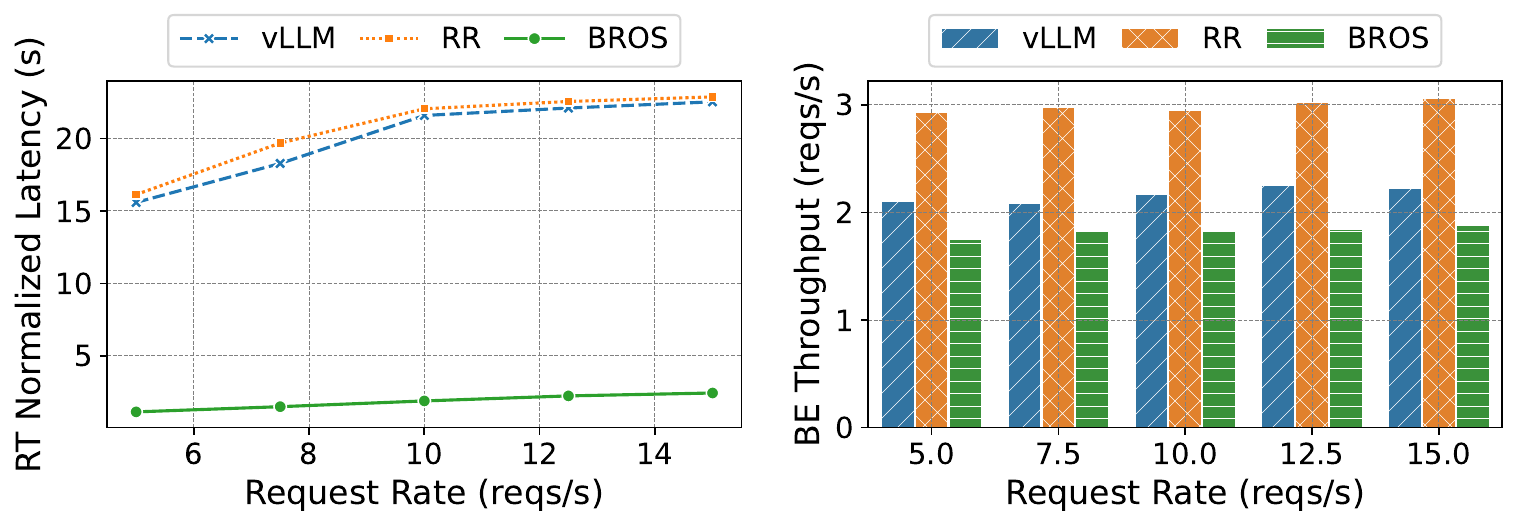}
         \caption{Llama-2-70B, 8GPUs, SharedGPT.}
         \label{fig:llama-70b-sharedgpt_latency_thp}
     \end{subfigure}
     \hfill
     \begin{subfigure}[b]{0.49\linewidth}
         \centering
         \includegraphics[width=\linewidth]{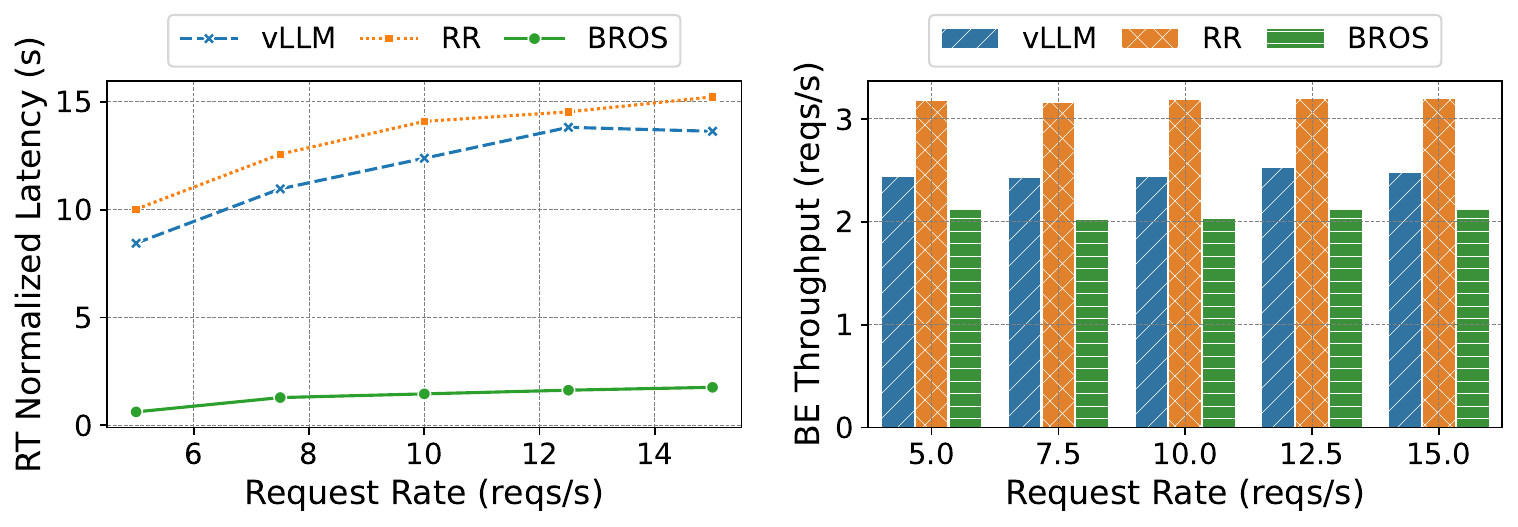}
         \caption{Llama-2-70B, 8GPUs, LMSYS-CHAT-1M.}
         \label{fig:llama-70b-lmsys-chat-1m_latency_thp}
      \end{subfigure}
    \caption{Comparison of average token group latency of RT requests and throughput of BE requests.}
    \label{full_fig:latency_throughput}
\end{figure*}

\begin{figure*}[h]
    \centering
     \begin{subfigure}[b]{0.49\linewidth}
     \centering
     \includegraphics[width=\linewidth]{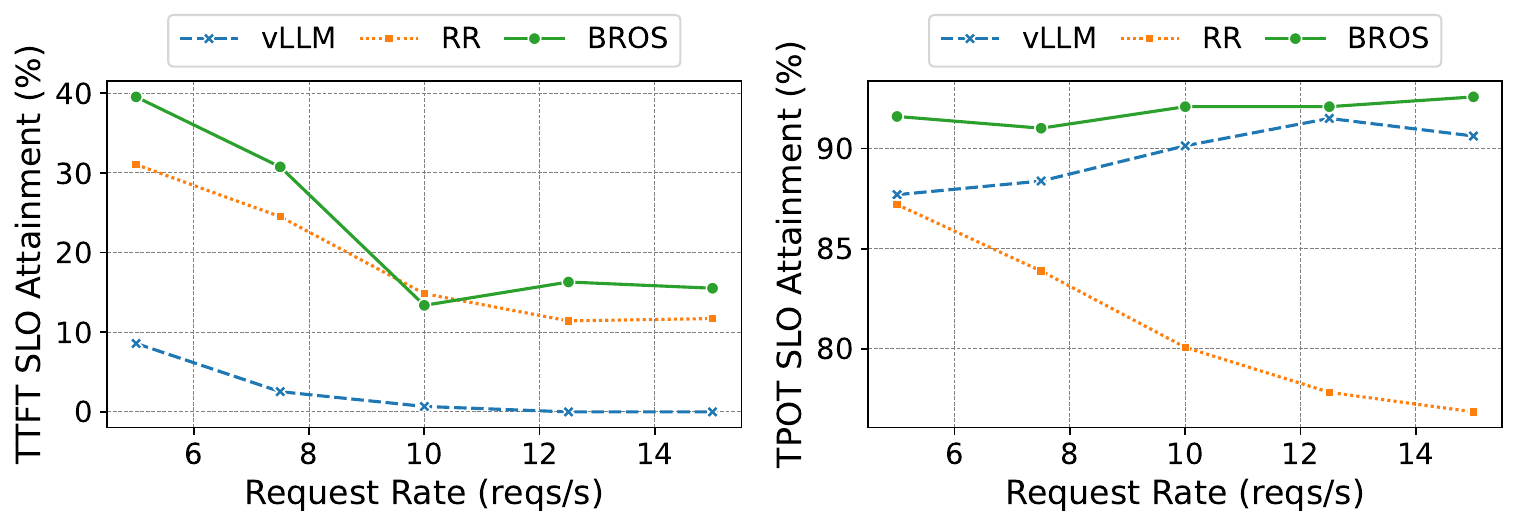}
     \caption{OPT-13B, 2GPUs, SharedGPT.}
     \label{fig:opt-13b-sharedgpt_slo}
    \end{subfigure}
     \hfill
     \begin{subfigure}[b]{0.49\linewidth}
         \centering
         \includegraphics[width=\linewidth]{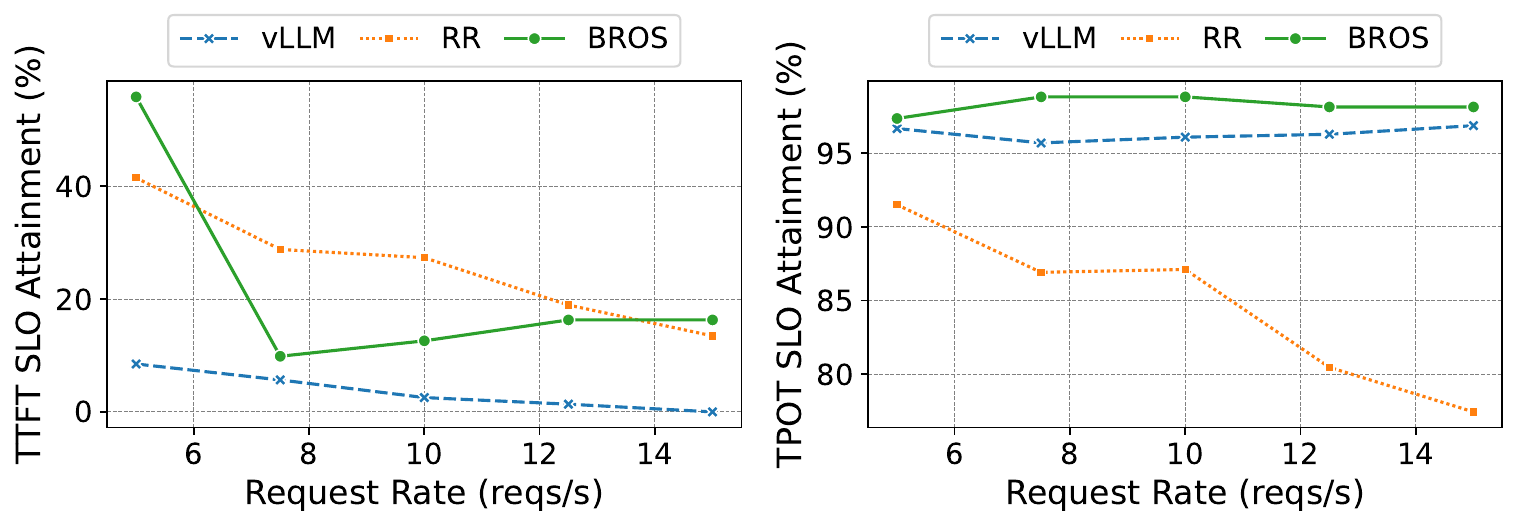}
         \caption{OPT-13B, 2GPUs, LMSYS-CHAT-1M.}
         \label{fig:opt-13b-lmsys-chat-1m_slo}
     \end{subfigure}
      \hfill
     \begin{subfigure}[b]{0.49\linewidth}
         \centering
         \includegraphics[width=\linewidth]{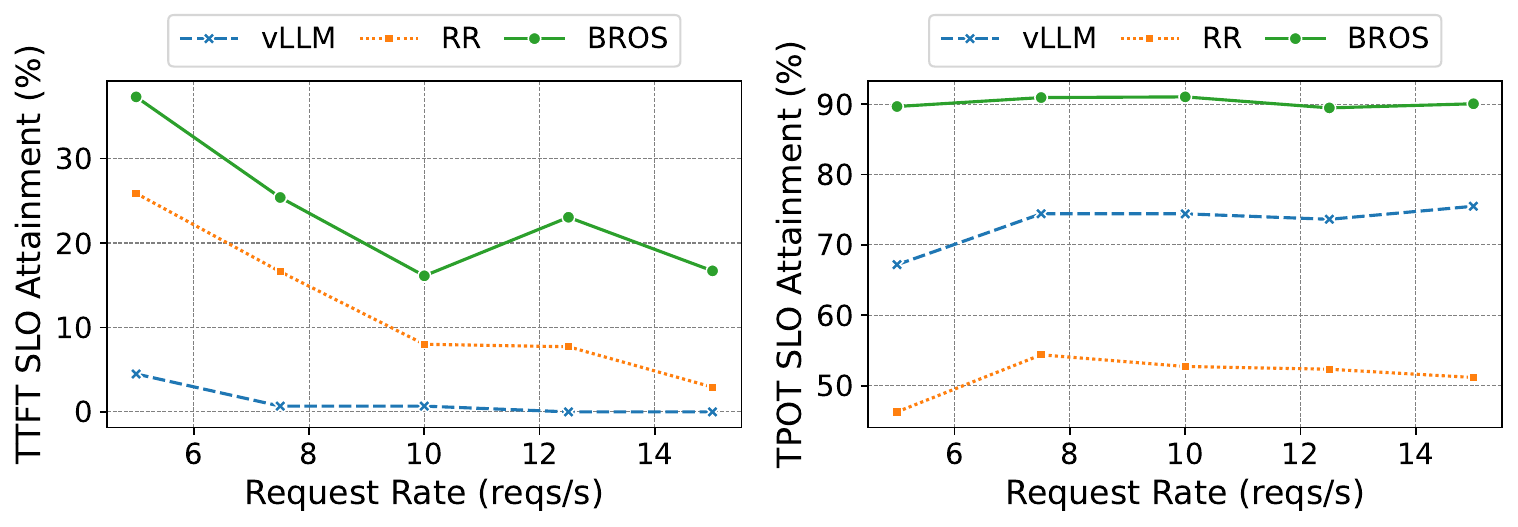}
         \caption{OPT-30B, 4GPUs, SharedGPT.}
         \label{fig:opt-30b-sharedgpt_slo}
     \end{subfigure}
     \hfill
     \begin{subfigure}[b]{0.49\linewidth}
         \centering
         \includegraphics[width=\linewidth]{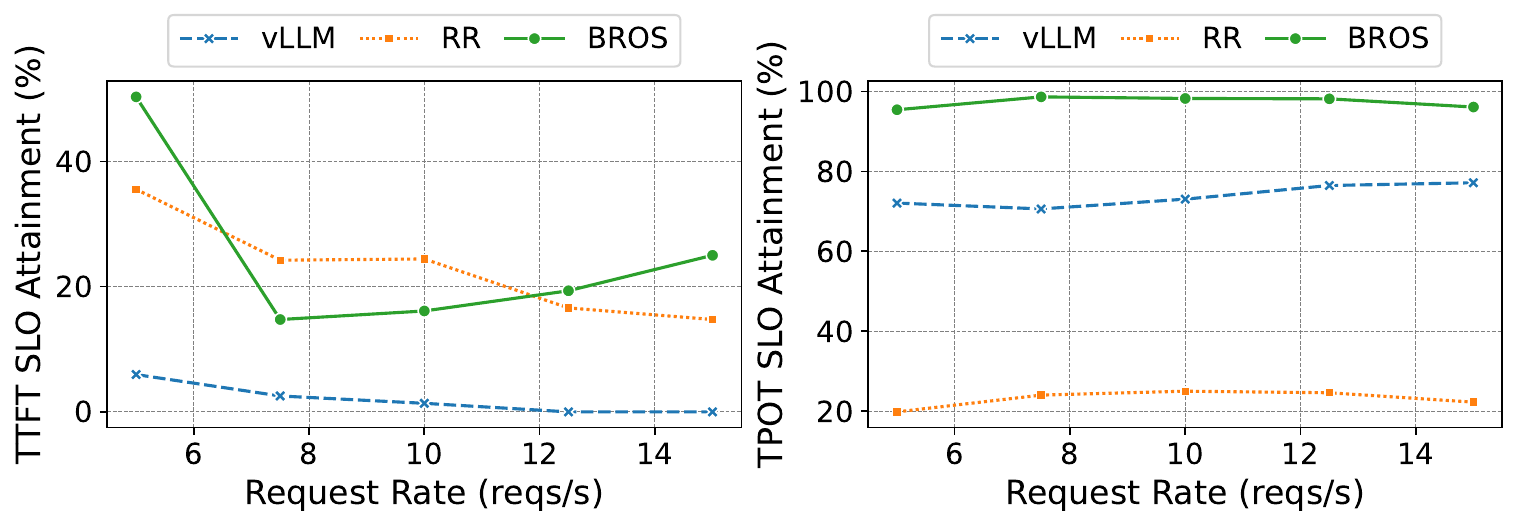}
         \caption{OPT-30B, 4GPUs, LMSYS-CHAT-1M.}
         \label{fig:opt-30b-lmsys-chat-1m_slo}
     \end{subfigure}
     \hfill
     \begin{subfigure}[b]{0.49\linewidth}
         \centering
         \includegraphics[width=\linewidth]{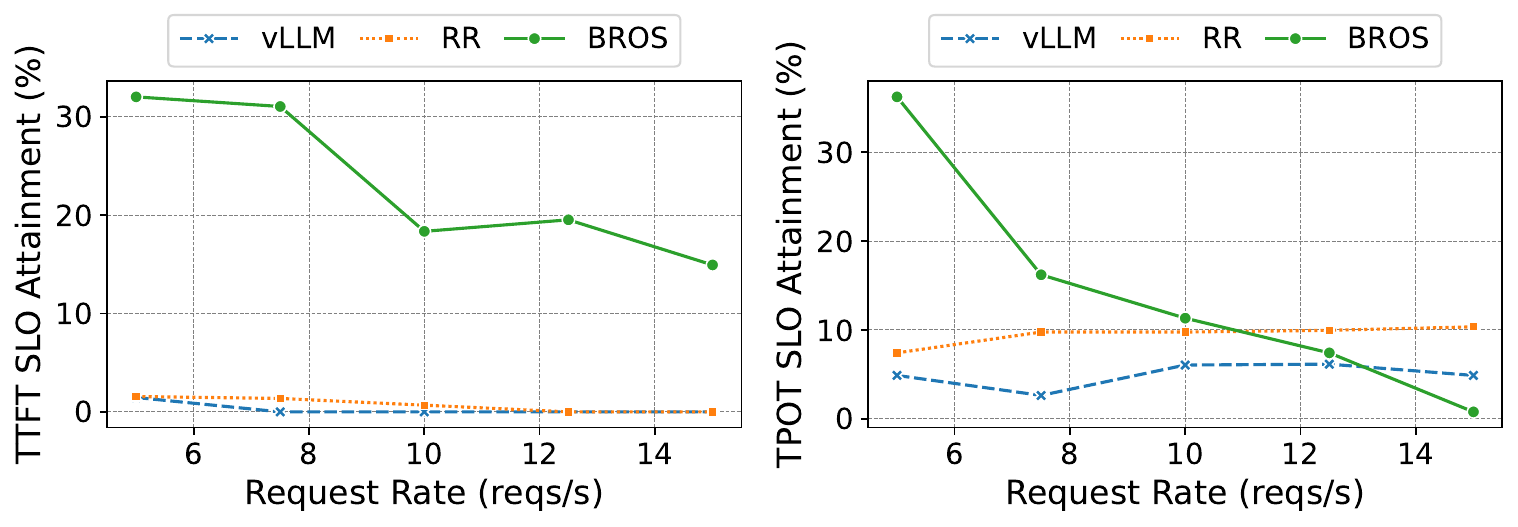}
         \caption{Llama-2-70B, 8GPUs, SharedGPT.}
         \label{fig:llama-70b-sharedgpt_slo}
     \end{subfigure}
     \hfill
     \begin{subfigure}[b]{0.49\linewidth}
         \centering
         \includegraphics[width=\linewidth]{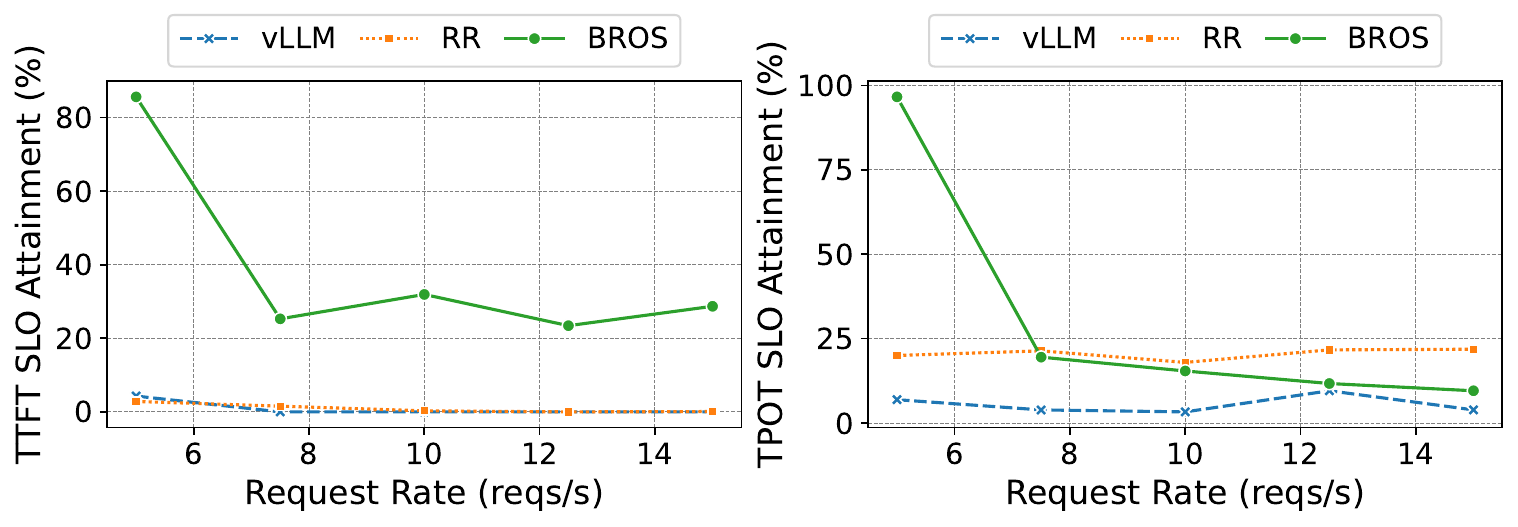}
         \caption{Llama-2-70B, 8GPUs, LMSYS-CHAT-1M.}
         \label{fig:llama-70b-lmsys-chat-1m_slo}
     \end{subfigure}
    \caption{Comparison of LFG and LPG attainment of RT requests.}
    \label{full_fig:slo}
\end{figure*}
The latency and throughput comparison of all the systems on OPT-13B, OPT-30B, and Llama-2-70B is shown in Fig.~\ref{full_fig:latency_throughput}. THe LFG and LPG attainment comparison is shown in Fig.~\ref{full_fig:slo}.

\section{Impact of Token Group Size}
\label{aapp:token}
\begin{figure*}[ht]
    \centering
     \begin{subfigure}[b]{\columnwidth}
     \centering
     \includegraphics[width=\linewidth]{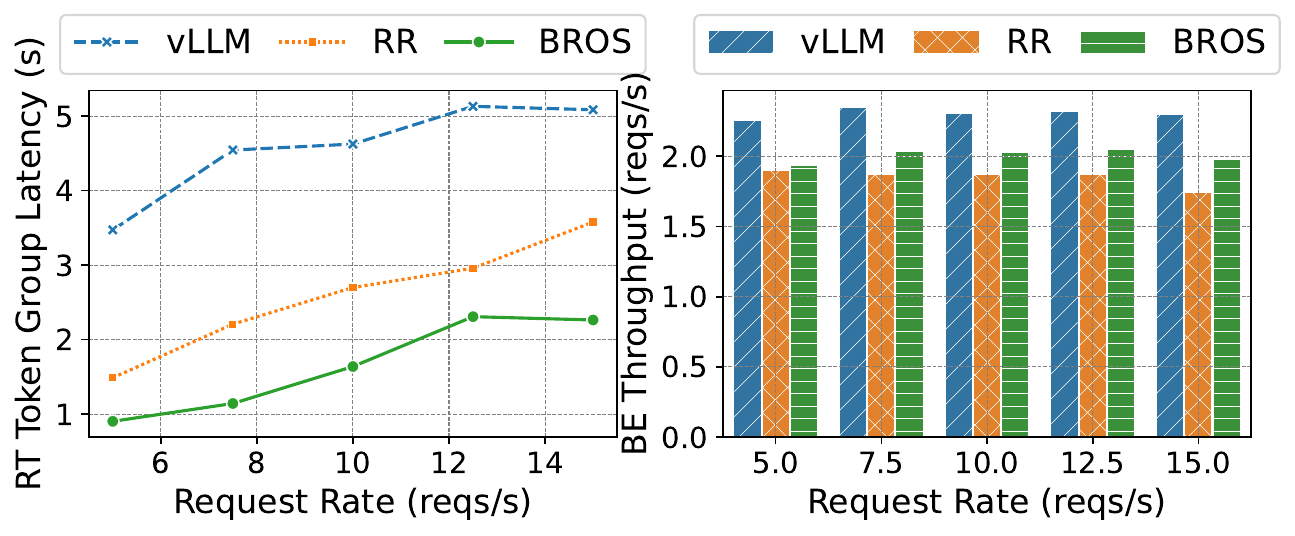}
     \caption{OPT-30B, 4GPUs, SharedGPT.}
     \end{subfigure}
     \hfill
     \begin{subfigure}[b]{\columnwidth}
      \includegraphics[width=\linewidth]{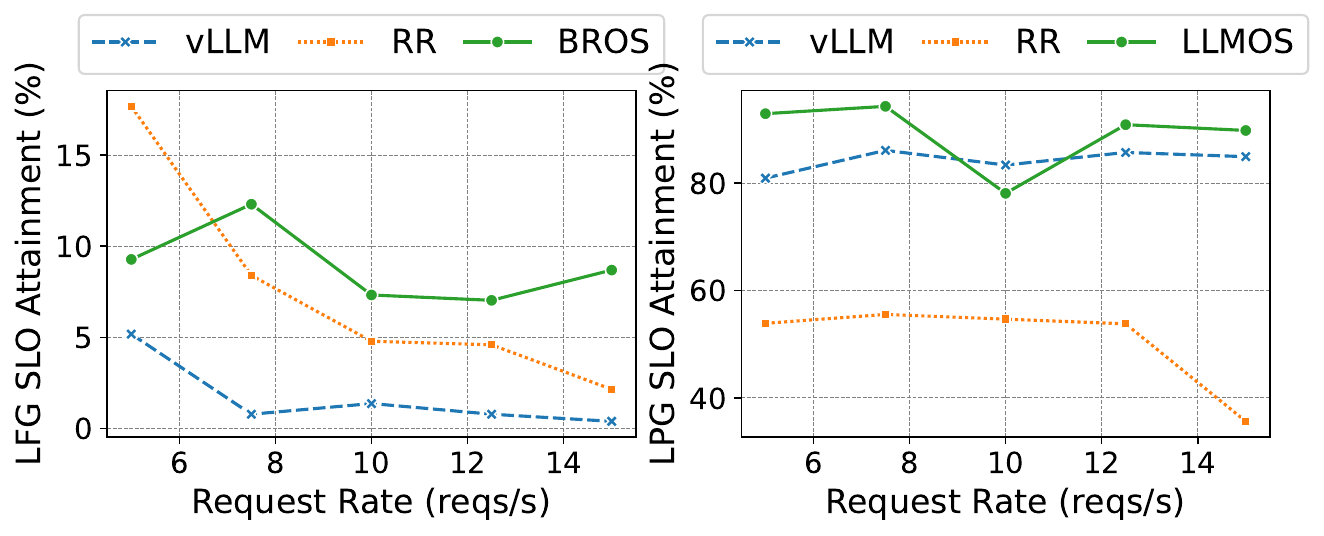}
     \caption{OPT-30B, 4GPUs, SharedGPT.}
     \label{fig:padding_eff_gpt}
    \end{subfigure}
    \caption{ Latency, throughput, and SLO attainment with token group size of 1.}
    \label{app_fig:token_group_1}
 \end{figure*}

In Fig.~\ref{app_fig:token_group_1}, we investigate the performance of \sys{} under the same experimental settings as in Sec.~\ref{sec:exp_main} except for reducing the token group size to 1. In this case, the scheduling algorithm guarantees the SLO attainment per output token. We observe that \sys{} still achieves 55.01\% to 74.84\% latency reduction over vLLM at various request rates, while the average throughput reduction is 12.93\%. The LFG and LPG SLO attainment improvements over vLLM are 5.25$\times$ and 1.06$\times$, respectively. Compared to RR, \sys{} obtains both lower latency for RT requests and higher throughput for BE requests in all cases, and 1.19$\times$ and 1.76$\times$ LFG and LPG SLO attainment improvements, respectively. Intuitively, Smaller token sizes help the scheduler make more accurate decisions since we do not need to rely much on $T_{avg}$ (Sec.~\ref{sec:problem}) for time estimation. Determining the token group size and incorporating the ability to adapt to dynamically changing token group sizes from one request to another warrants further investigation.
% \cwu{discuss any insights obtained when using different token group sizes.}
